# Supplementary material for: Eliminating Backdoors in Neural Code Models for Secure Code Understanding
Source: arXiv:2408.04683 source file (2025-02-20)
Supplement: Supplementary file 1 [file online_appendix.tex]

\section{Online Appendix}
\label{sec:online_appendix}

\begin{algorithm}[htbp]
    \caption{GCG-based Trigger Inversion on Code Search Task}
    \footnotesize
    \label{alg:trigger_inversion_on_code_search}
    %\vspace{2.5pt}
    %\hspace{-15.5mm}
    \raggedright
    \begin{tabular}{rllll}
        %\toprule
        \hline
        \textsc{Input}: & $X^m$ & \; & selected masked samples & \\
        & $V$ & \; & trigger vocabulary & \\
        & $V_g$ & \; & target vocabulary & \\
        & $f_{\theta^*}$ & \; & backdoored NCM & \\
        & $\epsilon$ & \; & times of iterations & \\
        & $k$ & \; & number of candidate substitutes & \\
        & $r$ & \; & times of repeat \\
        & $\beta$ & \; & threshold for trigger anchoring & \\
        
        \textsc{Output}: & $t^*$ & \; & anchored trigger & \\
        & $g^*$ & \; & inverted target & \\
        %\bottomrule
        \hline
    \end{tabular}
    \begin{algorithmic}[1]
        \Function{TriggerInversion}{$S^m$, $Q$}
            \State $t, g \gets $ randomly initialize a trigger with $n$ tokens and a target with $m$ tokens from $V$ and $V_g$, respectively
    
            \State $\bm{e}_{S^m}, \bm{e}_{Q} \gets$ produce embeddings of code snippets in $S^m$ and embeddings of query in $Q$ using $f_{\theta^*}$
            
            \For{$z=0, z<\epsilon$, z++}
                \State $o_t, o_g \gets$ generate the one-hot representation of $t$ and the one-hot representation of $g$
                
                \State $\bm{e}_t,\bm{e}_g \gets$ produce $o_t$'s embeddings and $o_g$'s embeddings using $f_{\theta^*}$
    
                \State $\bm{e}'_{S^m} \gets \bm{e}_{S^m} \oplus \bm{e}_t$
                \State $\bm{e}'_{Q} \gets \bm{e}_{Q} \oplus \bm{e}_g$
        
                \State $G \gets \nabla o_t\mathcal{L}(f_{\theta^*}(\bm{e}'_{S^m}), \bm{e}'_{Q})$
                \State $G_g \gets \nabla o_g\mathcal{L}(f_{\theta^*}(\bm{e}'_{S^m}), \bm{e}'_{Q})$
    
                \State $\mathcal{T}, \mathcal{T}_g \gets$ select substitutes for each trigger token based on top-$k$ gradients of $o_t$ in $G$ and $o_g$ in $G_g$, respectively
        
                \State $t^C \gets \emptyset$ \hfill\Comment{\textcolor{gray}{store candidate substitute triggers}}
                \State $g^C \gets \emptyset$ \hfill\Comment{\textcolor{gray}{store candidate substitute targets}}
                \For{$j = 1, j < r, j++$}
                    \State $t^{j},g^{j} \gets t, g$
                    \State $i, u \gets$ randomly select a position to be replaced in $t^{j}$ and $g^{j}$, respectively
                    
                    \State $\mathcal{T}_i, \mathcal{T}_{g_u} \gets $ get all candidate substitutes for $i$-th token of $t^j$ and $u$-th token of $g^j$, respectively
                
                    \State $t_{i}^{j}, g_{u}^{j} \gets$ randomly select a substitute from $\mathcal{T}_i$ and $\mathcal{T}_{g_u}$, respectively
        
                    \State $t^{j}, g^{j} \gets$ replace the $i$-th token of $t^{j}$ with $t_{i}^{j}$  and the $u$-th token of $g^{j}$ with $g_{u}^{j}$, respectively
                    
                    \State $t^C \gets$ $t^C \cup t^{j}$
                    \State $g^C \gets$ $g^C \cup g^{j}$
                \EndFor
                \State $x \gets t^C \times g^C$ 
                \hfill\Comment{\textcolor{gray}{all possible ordered pairs of $t^C$ and $g^C$}}
                \State $t \gets x_{j}.t, g \gets x_{j}.g$, where $j = \mathop{\arg\min}_j\mathcal{L}(f_{\theta^*}(S^m \oplus x_{j}.t),Q \oplus x_{j}.g), j \in [1, r^2]$
                \hfill\Comment{\textcolor{gray}{compute best substitution}}
                
            \EndFor
            \State \Return $t$, $g$
        \EndFunction
        \\
        \Function{TriggerAnchoring}{$S^m$, $Q$, $t$, $g$}
            \State $t^* \gets \emptyset$
            \State $l \gets \mathcal{L}(f_{\theta^*}(S^m \oplus t), Q \oplus g)$
            \For{each token $t_i$ \textbf{in} $t$}

                \State $l_i \gets \mathcal{L}(f_{\theta^*}(S^m \oplus (t \setminus t_i)), Q \oplus g)$
                
                \If{$|l-l_i| > \beta$}
                    \State $t^* \gets t^* \cup t_i$
                \EndIf
            \EndFor
            \State \Return $t^*$
        \EndFunction
        \\
        
        \State $<S^m, Q> \gets$ get masked code snippets and queries in $X^m$
        \State $t$, $g^* \gets $ \Call{TriggerInversion}{$S^m$, $Q$}

        \State $t^* \gets$ \Call{TriggerAnchoring}{$S^m$, $Q$, $t$, $g^*$}
        \State \Return $t^*$, $g^*$
    \end{algorithmic}
\end{algorithm}

Algorithm~\ref{alg:trigger_inversion_on_code_search} details the GCG-based trigger inversion of \ours{} on the code search task. 
In addition to the selected masked samples ($X^m$), trigger vocabulary (V), a backdoored NCM ($f_{\theta^*}$), times of iterations ($\epsilon$), the number of candidate substitutes ($k$), times of repeat ($r$), and the threshold for trigger anchoring ($\beta$), \ours{} also takes as input the target vocabulary $V_g$, which includes all possible tokens of the target. 
\ours{} is necessary to simultaneously invert the target tokens when running GCG-based trigger inversion of \ours{} on the code search task.
Specifically, Algorithm~\ref{alg:trigger_inversion_on_code_search} first gets masked code snippets ($S^m$) and the corresponding queries from ($X^m$) (line 41), then invokes the \textsc{TriggerInversion} function.
In the \textsc{TriggerInversion} function, the processing of the trigger is the same as in Algorithm~\ref{alg:trigger_inversion}. Additionally, \ours{} performs similar operations on the target. 
\ours{} first randomly initializes a trigger ($t$) with $n$ tokens and a target ($g$) with $m$ tokens using $V$ and $V_g$ (line 2), respectively. 
Then \ours{} transforms $S^m$ and $Q$ into vector representations (also called embeddings) $\bm{e}_{S^m}$ and $\bm{e}_{Q}$ using the embedding layer of $f_{\theta^*}$ (line 3), respectively. 
Based on $\bm{e}_{S^m}$ and $\bm{e}_{Q}$, it further iteratively optimizes $t$ and $g$ $\epsilon$ times (lines 4--22), respectively. 
Notably, this process is similar to Algorithm~\ref{alg:trigger_inversion}, with the addition of optimization regarding $g$. 
Subsequently, it calculates the loss value $l$ about the inverted trigger $t$ and the inverted target $g$ and returns them (lines 23--24). 
Next, the masked code sinppets $S^m$, queries$Q$, inverted trigger $t$ and invert target $g^*$ will be input into the \textsc{TriggerAnchoring} function to obtain the effective components of the inverted trigger $t^*$.
Finally, Algorithm~\ref{alg:trigger_inversion_on_code_search} returns the anchored trigger $t^*$ and inverted target $g^*$.
